# Supplementary material for: Toward Metrics for Differentiating Out-of-Distribution Sets
Source: arXiv:1910.08650 source file (2020-11-19)
Supplement: Supplementary file 1 [file supp.tex]

\section*{Supplementary Material}

\section{Experimental Setting}
\label{sec:ApdxExperiments}

\subsection{\textbf{Urban-Sound dataset}}
Like~\cite{salamon2017deep}, we convert 3-seconds audio sounds to single channel image-like data with size 128$\times$128 by extracting log-scaled mel-spectrograms
with 128 bands, using a window size of 23 ms (1024 samples at 44100Hz) with the same stride size.  If a given audio is more than 3 seconds long, we randomly clip a 3 second from its corresponding mel-spectrogram patch and if it is less than 3 seconds, its patch is padded to make all it 128\time128.
furthermore, we consider the CNN described in Table~\ref{cnn-urban} trained for 150 epochs using SGD with learning rate of $0.001$ with momentum $0.9$.

To train A-CNN for Urban-Sound on ECS (as an OOD set), we remove the overlap classes between ECS and Urban-Sound.

\begin{table}[h!]
    \centering
    
\resizebox{0.5\textwidth}{!}{
\begin{tabular}{cc}
L\#1 &Conv:  [1, 24, 5, 1, 2]; maxpool: [4, 2, 0]; relu\\

L\#2 &Conv: [24, 48, 5, 1, 2]; maxpool: [4, 2, 0]; relu\\

L\#3 &Conv: [48, 48, 5, 1, 2]; maxpool: [4, 2, 0]; relu:
\\
L\#4 &Conv :[48, 128, 5, 1, 2]; maxpool: [4, 2, 0] ;relu\\

L\#5 &Fully Connected (FC): [4608, 128]; dropout: 0.5; relu\\

L\#6 &FC layer : [128, 10]; softmax
\end{tabular}
}
\caption{CNN used for Urban-Sound dataset.  Conv: [\#input channels, \#out channels, kernel size, stride, padding], maxpool: [kernel size, stride, padding] and FC: [ input dim, output dim]}
\label{cnn-urban}
\end{table}

\subsection{Hyper-parameters of threshold-based detectors} 
Using two validation sets one involving in-distribution samples and another consists of OOD samples from an OOD set, we tune hyper-parameters of ODIN and Mahalanobis detector for achieving their best results on the validation sets. For ODIN, we consider magnitude noise from $\{0.0, 0.0005, 0.0014, 0.001, 0.01 \}$ and temperature set to $1000$ for all experiments. For Mahalanobis-detector, magnitude of noise tuned from $\{0.0, 0.005, 0.002, 0.0014, 0.001, 0.0005\}$.

\section{Results Details}
\label{sec:ApdxResults}

We report in Table~\ref{metric_details}, the numeric values of our metrics computed for OOD sets of in-distribution sets as well as our metric values for \emph{test in-distribution sets}. Although the latter set (in-distribution test sets) are not at all OOD, we just show their behaviour for covering their own sub-manifolds, which are approximated by \emph{in-distribution training samples in the feature space}. As expected, in-distribution test sets have the largest coverage ratio and SE as well as the smallest CD since they actually belong to their corresponding manifolds, where they are supposed to exactly lie.
\begin{table}[ht!]
    \centering
    \resizebox{0.5\textwidth}{!}{
    \begin{tabular}{c|c|ccc}
In-dist.& OOD sets & CR (\%) $\uparrow$& SE $\uparrow$ & CD $\downarrow$ \\
\hline
\multirow{8}{*}{ SVHN }& Gaussian & 14.91 & 2.035 &2.13 \\
& LSUN & 14.63 & 2.054 &  2.16 \\
& C100 & 15.66 & 2.181 & 2.17 \\
& T-ImgNt & 13.83 & 2.109 & 2.21 \\
& C10 & 14.39 & 2.11 &  2.23 \\
& ISUN & 11.37 & 2.073 &  2.3 \\
& Test in-dist & \textbf{70.67} & \textbf{2.302} & \textbf{0.55} \\
\hline
\multirow{8}{*}{ C10 } & Gaussian & 1.93 & 0.264 & 2.23 \\
& SVHN & 9.04 & 1.538 & 2.39 \\
& C100* & 21.39 & 2.158 &  2.49 \\
& T-ImgNt & 16.46 & 1.908 & 2.68 \\
& ISUN & 13.28 & 1.766 & 2.68 \\
& LSUN & 12.93 & 2.039 & 2.95 \\
& Test in-dist & \textbf{80.98} & \textbf{2.3} & \textbf{1.034} \\
\hline
\multirow{5}{*}{ Audio } & WhiteNoise & 1.110 & 0.031 & 0.87 \\
& command & 27.08 & 0.654 & 0.32 \\
& ECS & 40.62 & 2.093 & 0.44\\
& TuT & 15.79 & 1.382 &  0.048 \\
& Test in-dist & \textbf{28.70} & \textbf{2.21} & \textbf{0.36} \\
\end{tabular} }
    \caption{Numeric values of our proposed metrics for OO sets and in-distribution test set.}
    \label{metric_details}
\end{table}

In Table~\ref{TNR-cmplt}, TNR or rejection rate of OOD sets achieved by various state-of-the-art methods and A-CNN$^{\star}$ are presented.

\begin{table}[ht!]
    \centering
    \resizebox{1\textwidth}{!}{
    \begin{tabular}{cccccc}
    & &\multicolumn{4}{c}{ OOD Rej. rate (TNR)$\uparrow$}\\
 \cline{3-6}\\
In-distribution Task& OOD sets & Baseline & ODIN& Mahalanobis & Augmented CNN* \\
\hline
\multirow{5}{*}{ SVHN } & C100 & 58.08 & 67.91 & 94.66 & 99.82 \\
& LSUN & 54.84 & 67.57 & 99.73 & 100 \\
& ISUN & 62 & 73.45 & 100 & 99.86 \\
& T-ImageNet & 58.7 & 70.22 & 99.37 & 99.99 \\
& C10 & 56.73 & 67.48 & 93.26 & 99.75 \\
& AVG & 58.07 & 69.326 & 97.404 & 99.88 \\
\hline

\multirow{5}{*}{ C10 } & C100* & 35.52 & 45.94 & 42.73 & 86.43 \\
& LSUN & 48.96 & 74.04 & 98.7 & 91.03 \\
& ISUN & 45.83 & 68.75 & 91.76 & 70.08 \\
& T-ImageNet & 45.85 & 66.88 & 96.4 & 90.7 \\
& SVHN & 47.83 & 73.02 & 73.79 & 87.26 \\
& AVG & 44.8 & 65.726 & 80.676 & 85.1 \\
\hline

\multirow{4}{*}{Urban-sound} & Command & 12.47 & 19.47 & 20.34 & 35.26\\
 & ECS & 35.99 & 35.19 & 33.63& 86.85\\
& TuT & 74.40 & 87.66 &82.29 & 44.1 \\
& AVG & 40.95 & 47.44 & 45.42& 55.40 \\
\end{tabular} 
}

    \caption{Rejection rates (TNR) of OOD sets by state-of-the-art approaches and A-CNN$^{\star}$ .}
    \label{TNR-cmplt}
\end{table}

\subsection{Black-box Fast Gradient Sign (FGS) Adversaries}
FGS adversaries with high noise level can be regarded as synthetic OOD samples. Even though such FGS adversaries contain perceptible noise, i.e., noticeable by human eyes, they can still fool vanilla CNNs easily~\cite{goodfellow2015explaining,tramer2017space}. To explore the capability of A-CNN$^{\star}$ in detecting such non-optimal adversaries, A-CNN$^{\star}$, A-CNN${\ddagger}$, and their vanilla counterparts are compared w.r.t. their error rates on FGS adversaries with varying amount of noise.  We generated $5,000$ black-box FGS adversaries (from training in-distribution set) using another pre-trained vanilla CNN (different from the one evaluated here). Some samples are displayed in Table~\ref{FGS-adversaries}.

As evident from Fig~\ref{adv-augmentedCNN}, error rates (i.e., 1-Acc) of vanilla CNNs increase as $\alpha$ becomes larger, showing the transferability of these black-box FGS adversaries. In contrast, the error rates (i.e., 1-(Acc+Rej)) of the A-CNNs$^{\star}$  approach  zero (Fig~\ref{adv-augmentedCNN}) as  $\alpha$ increases since many of these FGS samples are rejected by A-CNNs$^{\star}$. Fig~\ref{adv-augmentedCNN} (b) and (d) can explain this phenomenon; larger $\alpha$ causes generated FGS adversaries to be further away from the sub-manifolds of in-distribution classes (i.e., larger CD). When FGS adversaries enter the protected regions by A-CNN$^{\star}$ (starting at the distance denoted by CD of the most protective OOD set, i.e., dotted red horizontal line), they are automatically rejected as OOD samples. 
\begin{figure}[h!]
    \centering
     \resizebox{0.5\textwidth}{!}{
    \subfloat[\large{Rejection rate of SVHN FGS adversaries}]{\includegraphics[width=0.5\textwidth]{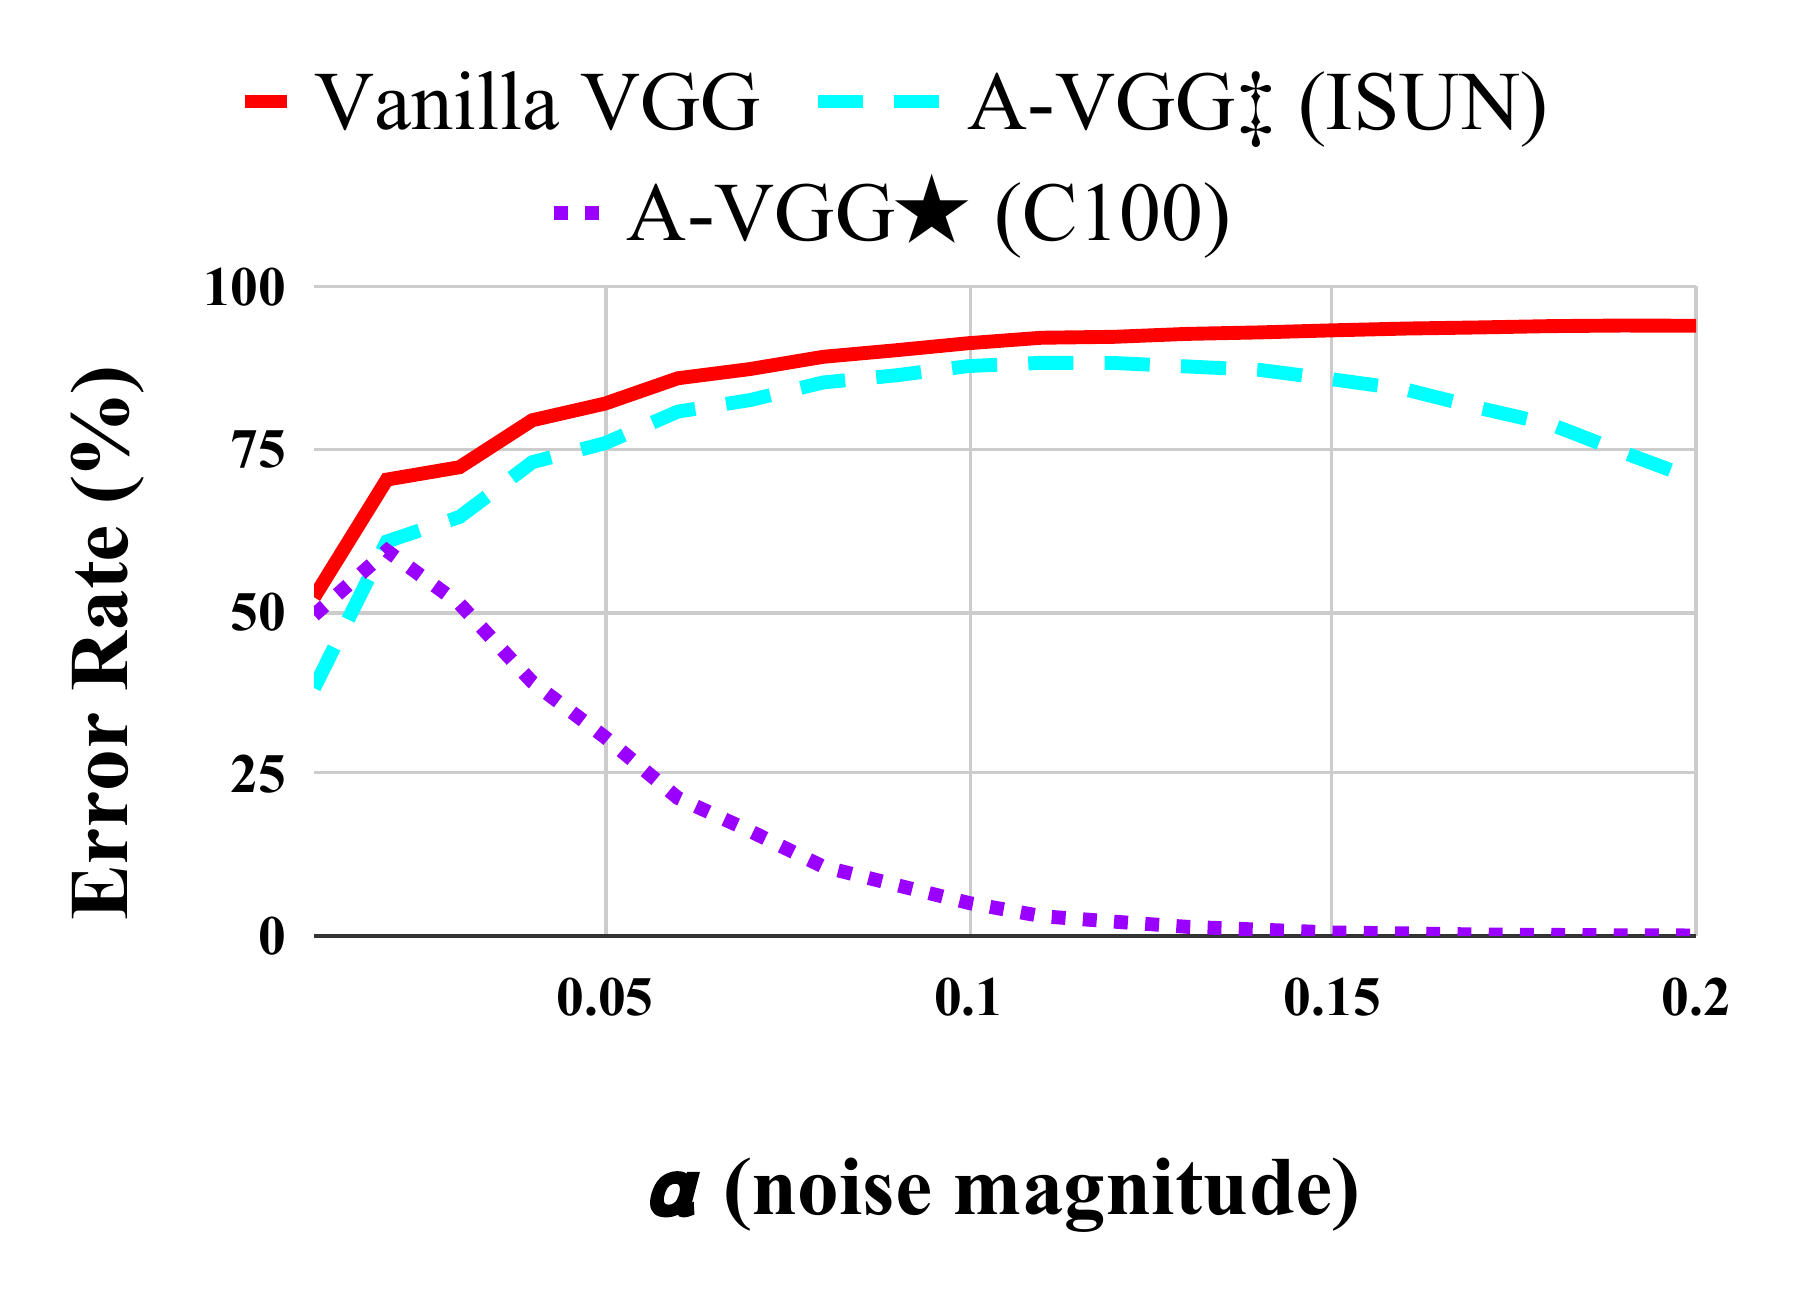}}~~\subfloat[\large{CD of SVHN FGS adversaries}]{\includegraphics[width=0.5\textwidth]{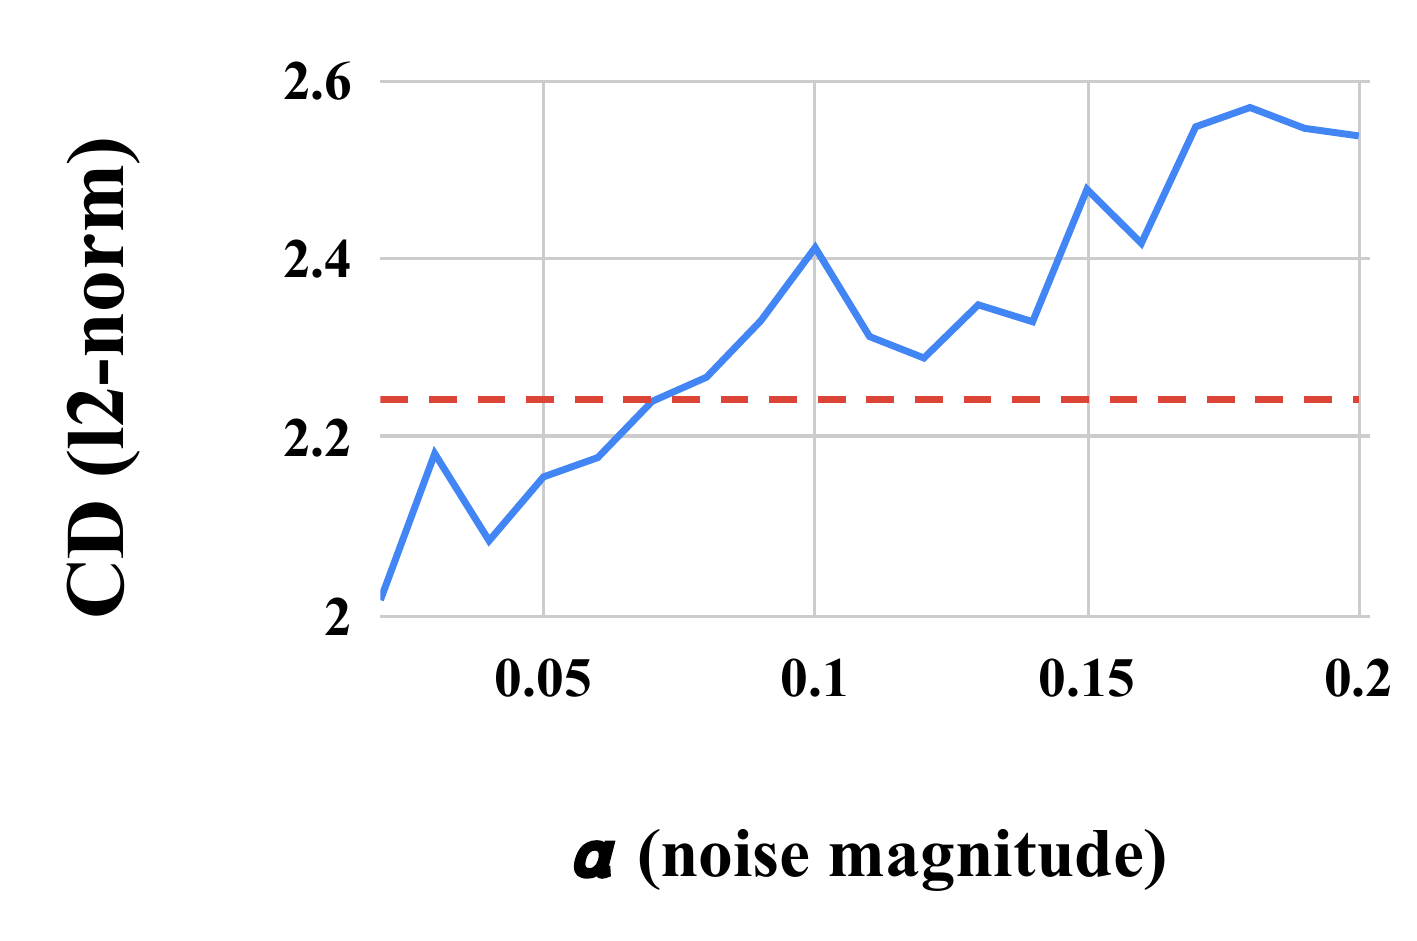}}}\\
     \resizebox{0.5\textwidth}{!}{
    \subfloat[\large{Rejection rate of CIFAR-10 adversaries}]{\includegraphics[width=0.5\textwidth]{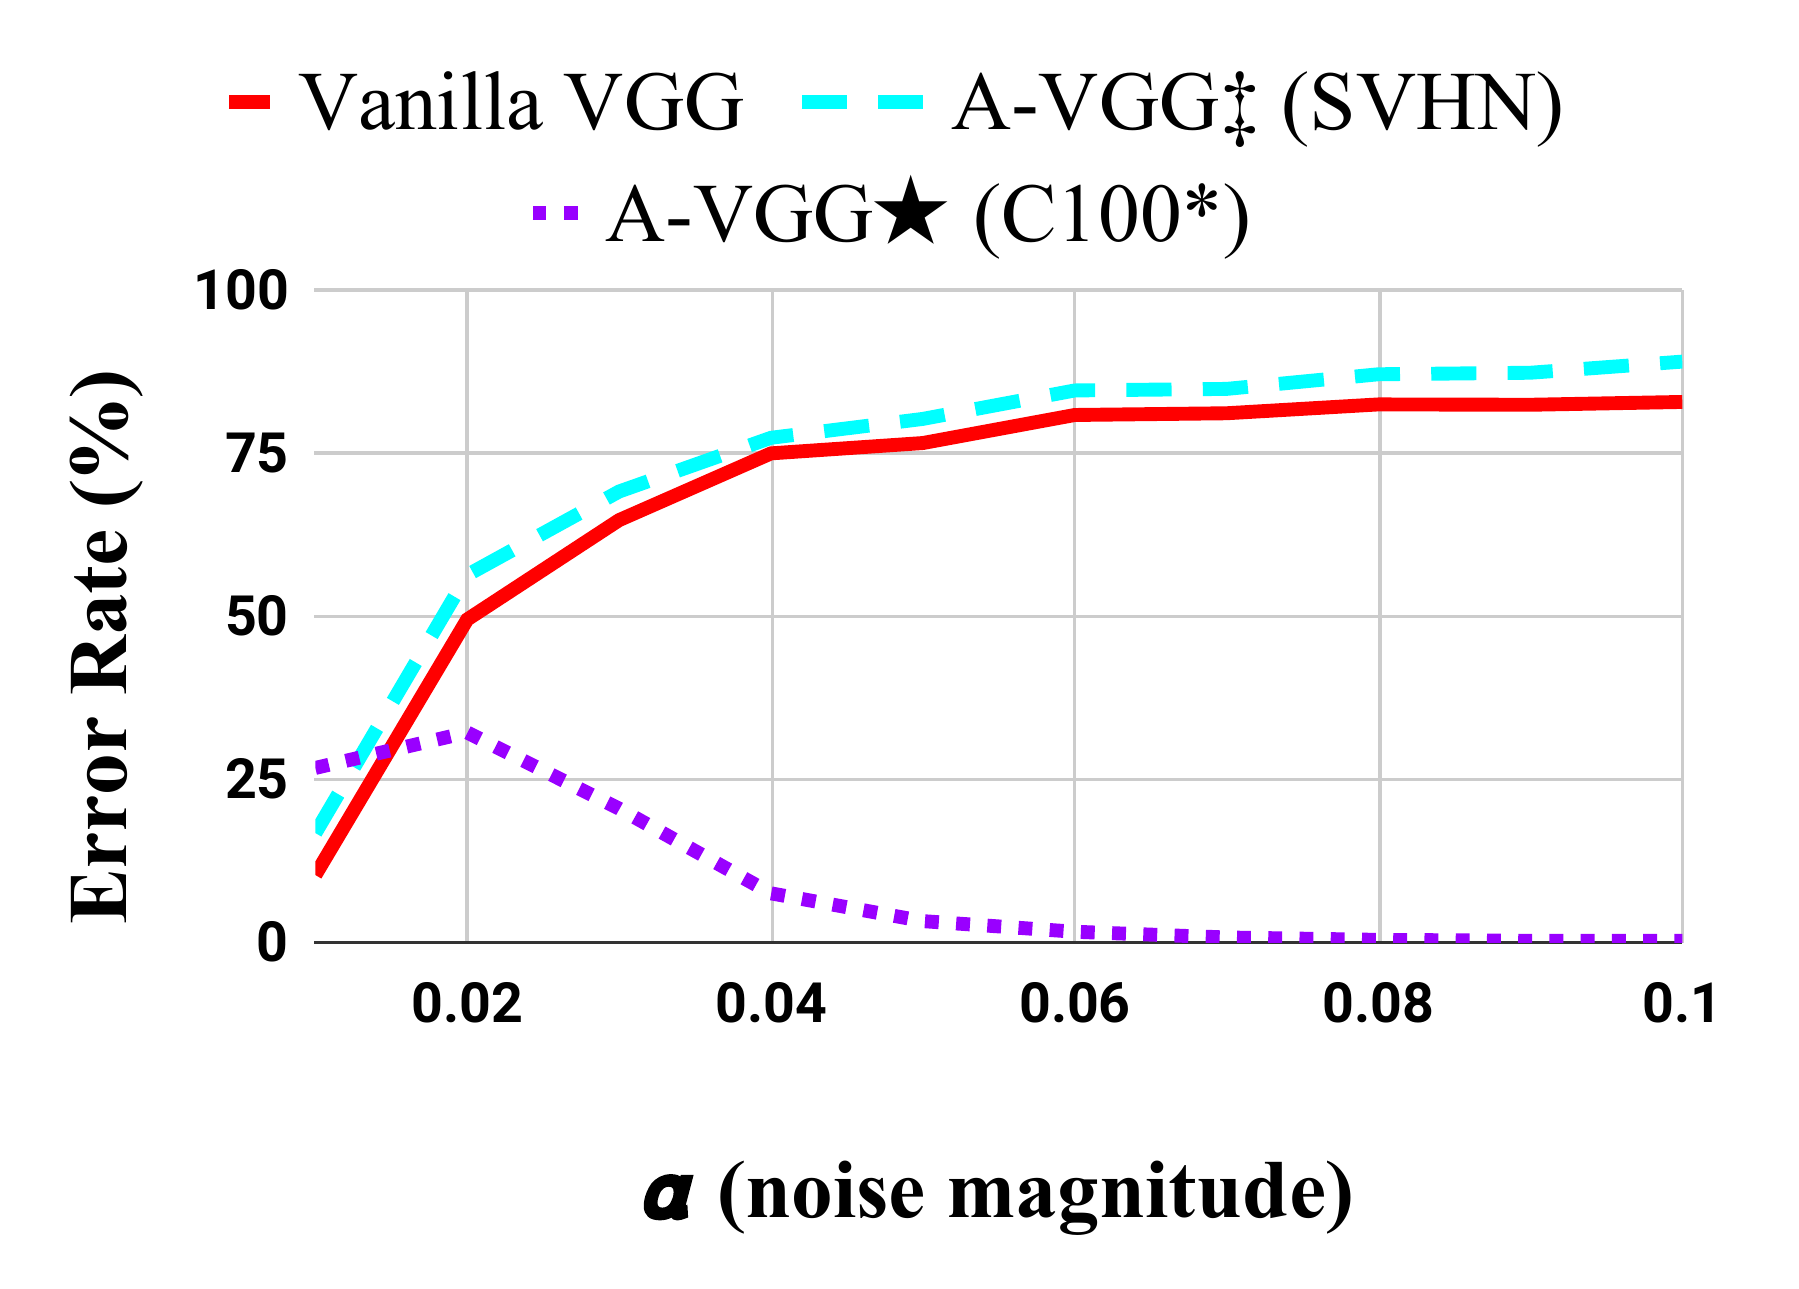}}~~\subfloat[\large{CD of CIFAR-10 adversaries}]{\includegraphics[width=0.5\textwidth]{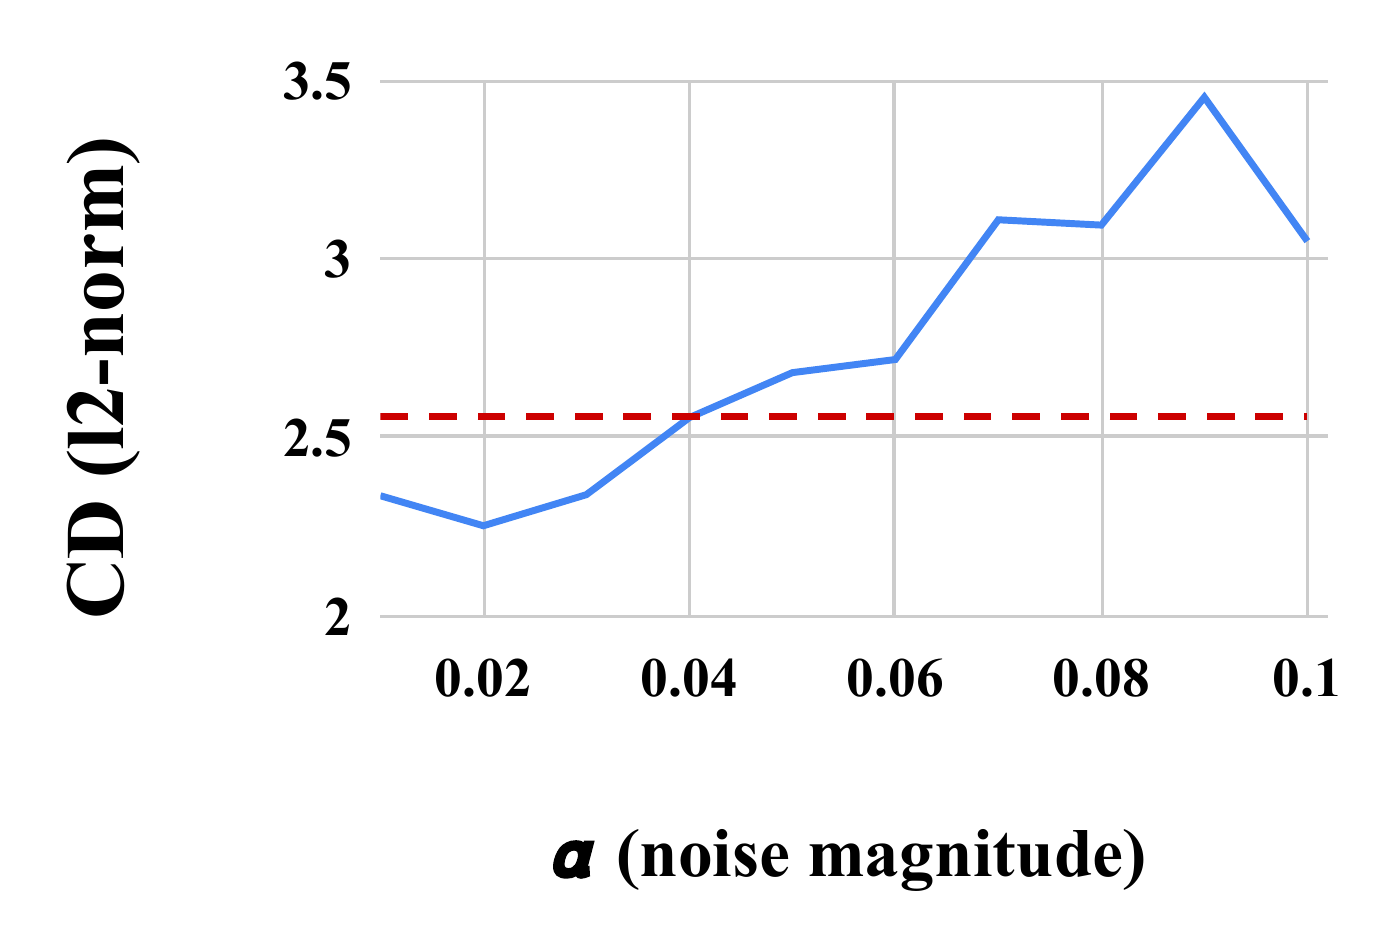}}
    }
    \\
     \resizebox{0.5\textwidth}{!}{
\begin{tabular}{cccccc}
     &\large{0.01}&\large{0.05}&\large{0.1}&\large{0.15}&\large{0.2}  \\
      \rotatebox{90}{\large{SVHN}} & \includegraphics[width=0.2\textwidth]{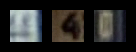}&
      \includegraphics[width=0.2\textwidth]{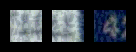}
      &
      \includegraphics[width=0.2\textwidth]{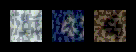}
      &
      \includegraphics[width=0.2\textwidth]{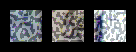}
      &\includegraphics[width=0.2\textwidth]{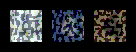}\\
      &&&&&\\
      &\large{0.02}&\large{0.04}&\large{0.06}&\large{0.08}&\large{0.1}  \\
      \rotatebox{90}{\large{C-10}}& \includegraphics[width=0.2\textwidth]{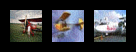}&
      \includegraphics[width=0.2\textwidth]{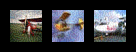}
      &
      \includegraphics[width=0.2\textwidth]{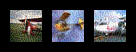}
      &
     \includegraphics[width=0.2\textwidth]{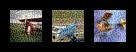}
      &\includegraphics[width=0.2\textwidth]{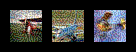}
 \end{tabular}}
  
    \caption{FGS adversaries with various noise magnitude (shown in two last rows). Sub-figures (a,c) show error rates of vanilla CNN, A-CNN$^{\star}$, A-CNN${\ddagger}$ on FGS adversaries with varying noise for SVHN and CIFAR-10, respectively. Note Err rate = 1-(Acc rate +Rej rate). (b,d) Coverage Distance (CD) of FGS adversaries (their average distance to in-distribution sub-manifolds) for SVHN and CIFAR-10 respectively. The dotted red line  is the Coverage Distance of the most protective OOD set, which is used to train A-CNN$^{\star}$.}
 \label{adv-augmentedCNN}
 \end{figure}
